# Supplementary material for: DFormer: Rethinking RGBD Representation Learning for Semantic Segmentation
Source: arXiv:2309.09668 source file (2024-02-07)
Supplement: Supplementary file 1 [file supp_SOD.tex]

\begin{table}[t]
\scriptsize
\setlength\tabcolsep{2.2pt}
\setlength\extrarowheight{1pt}
\begin{center}
\caption{Quantitative comparisons on RGB-D SOD benchmarks. The best results are \highlight{highlighted}. `-' means the results of some methods are not provided in their paper.
% We use the Mean Absolute Error ($M$), max F-measure ($F$), S-measure ($S$), and max E-measure ($E$) as evaluation metrics.
}
\vspace{-10pt}
\label{tab:sod_supp}
% \resizebox{0.99\linewidth}{!}{
\begin{tabular}{lcc|| llll|llll|llll}
\toprule
 Dataset & Param  & Flops &\multicolumn{4}{c}{DUTLF-Depth}  & \multicolumn{4}{c}{ReDWeb-S}   & \multicolumn{4}{c}{LFSD}  \\%& \multicolumn{4}{c}{SSD} \\
\cline{4-7} \cline{8-11} \cline{12-15} %\cline{22-25}

Metric & \makecell{(M)} &\makecell{(G)}& $M$ &  $F$  &  $S$ &  $E$  &  $M$ &  $F $  &  $S$ &  $E$  &  $M$ &  $F $  &  $S$ &  $E$  \\%&  $M$ &  $F $  &  $S$ &  $E$\\
\hline
%$CPFP_{19}$ & .038 & .846 & .872  &.923 & .036 & .867 & .888  &.932 & .053 & .877 & .878  &.923 & .051 & .874 & .879  &.925 & .064 & .851 & .850  &.903 \\%& .082 & .766 & .807  &.852 \\

BBSNet$_{21}$ (\citeauthor{zhai2021bifurcated})& 49.8& 31.3&.058&.870&.882&.912&.150&.680&.693&.763&.092&.828&.835&.870 \\%& .044 & .859 & .882  &.919 \\

DCF$_{21}$ (\citeauthor{ji2021calibrated}) & 108.5& 54.3&.030&.926&.929&.952&-&-&-&-&-&-&-&-\\

DSA2F$_{21}$ (\citeauthor{sun2021deep})& 36.5 & 172.7 &.030&.926&.921&.950&-&-&-&- &.054&.882&.882&.923  \\%& .045 & .852 & .846  &.904 \\
% DFMNet$_{21}$ (\citeauthor{Zhang2021DFMNet}) & - & - & .019 & .932 & .938  &.973 & .024 & .912 & .926  &.961 & .039 & .913 & .912  &.950 & .040 & .904 &.908  &.948 & .049 & .890 & .885  &.926 \\%& - & - & -  & - \\
% TriTrans$_{21}$(\citeauthor{}) & & & .014 & .946 & .943  &.978 & .020 & .930 & .928  &.963 & .030 & .934 & .920  &.953 & .033 & .920 & .908  &.949 & .043 & 916 & .886  &.928  \\ %& - & - & -  & - \\
CMINet$_{21}$ (\citeauthor{cascaded_cmi}) & - & - &-&-&-&-&-&-&-&-&.064&.862&.877&.911  \\%& - & - & -  & - \\
DSNet$_{21}$ (\citeauthor{wen2021dynamic}) & 172.4 &141.2&-&-&-&-&.133&.676&.716&.736&.068&.849&.867&.890 \\ 
UTANet$_{21}$ (\citeauthor{zhao2021rgb}) & 48.6& 27.4 &-&-&-&-&-&-&-&-&-&-&-&- \\%& .042 & .881 & .885  &- \\
BIANet$_{21}$ (\citeauthor{zhang2021bilateral}) & 49.6&59.9&-&-&-&-&-&-&-&-&-&-&-&-  \\
SPNet$_{21}$ (\citeauthor{zhou2021specificity})& 150.3&68.1&-&-&-&-&-&-&-&-&-&-&-&- \\ % & .044 & .883 & .871  & .915 \\
\rowcolor{gray!15}VST$_{21}$ (\citeauthor{liu2021visual})& 83.3 & 31.0&.024&.948&.943&.969&.113&.763&.759&.826&.061&.889&.882&.921 \\
\rowcolor{gray!15}RD3D+$_{22}$ (\citeauthor{chen20223})& 28.9 & 43.3&.030&.945&.936&.964&.130&.697&.718&.786&-&-&-&- \\
\rowcolor{gray!15}BPGNet$_{22}$ (\citeauthor{yang2022bi})&84.3&138.6&.031&.938&.930&.958&-&-&-&-&.066&.875&.874&.908 \\
% MobileSal$_{22}$ (\citeauthor{})\\
C2DFNet$_{22}$ (\citeauthor{zhang2022c}) & 47.5&21.0&.025&.934&.931&.958&-&-&-&-&.065&.863&.880&.883\\ 
MVSalNet$_{22}$ (\citeauthor{zhou2022mvsalnet})   & - &-&-&-&-&-&-&-&-&-&.072&.880&.856&.906  \\  
SPSN$_{22}$ (\citeauthor{lee2022spsn})  & 37.0& 100.3&-&-&-&-&-&-&-&-&-&-&-&-    \\   

% RFNet$_{22}$(\citeauthor{}) & 365 & &.015& .946& .941& .977
% &.020&.932&.931&.962
% & .029 & .936 &.926& .951 
% &.035&.921&.911& .944 
% &.042& .916 & .893 &.931 \\

HiDANet$_{23}$~(\citeauthor{wu2023hidanet})&  130.6&71.5&-&-&-&-&-&-&-&-&-&-&-&-  \\

\hline
% \rowcolor[RGB]{235,235,250 
\rowcolor{gray!15}\nMethod{}-T& 5.9 &4.5 &.027&.940&.935&.960&.115&.800&.747&.819&.059&.892&.876&.910  \\
\rowcolor{gray!15}\nMethod{}-S&18.5&10.1&.027&.942&.938&.963&.113&.802&.751&.821&.059&.895&.880&.913\\
\rowcolor{gray!15}\nMethod{}-B&29.3&16.7&.025&.945&.940&.966&.109&.809&.755&.823&.058&.899&.881&.920\\
\rowcolor{gray!15}\nMethod{}-L&38.8&26.2&\highlight{.023}&\highlight{.952}&\highlight{.945}&\highlight{.970}&\highlight{.106}&\highlight{.813}&\highlight{.760}&\highlight{.826}&\highlight{.056}&\highlight{.903}&\highlight{.885}&\highlight{.925}\\
\bottomrule
\end{tabular}
\vspace{-10pt}
\end{center}
\end{table}
